# Supplementary material for: Usability of Privacy Controls in Top Health Websites
Source: arXiv:2303.01838 source file (2023-03-03)
Supplement: Supplementary file 1 [file Appendix.tex]

\section{Appendix}
\label{sec:appendix}

\begin{table}[htb]
\caption{Top 100 Health Website Domain List}
\label{table:rank}
\footnotesize
\centering
\begin{tabular}{llllll}
\toprule
% \textbf{Regulation Abbreviation}&\textbf{Regulation Full Name}&\textbf{Country} \\
% \midrule

1	&	healthline.com	&	35	&	amboss.com	&	69	&	emergencyemail.org		\\
2	&	nih.gov	&	36	&	theessentialbs.com	&	70	&	zennioptical.com		\\
3	&	medicalnewstoday.com	&	37	&	kp.org	&	71	&	hopkinsmedicine.org		\\
4	&	webmd.com	&	38	&	pointclickcare.com	&	72	&	whattoexpect.com		\\
5	&	mayoclinic.org	&	39	&	verywellhealth.com	&	73	&	labcorp.com		\\
6	&	walgreens.com	&	40	&	psychologytoday.com	&	74	&	shop-apotheke.com		\\
7	&	cdc.gov	&	41	&	sportkp.ru	&	75	&	tabletki.ua		\\
8	&	doctolib.fr	&	42	&	youlai.cn	&	76	&	eapteka.ru		\\
9	&	tuasaude.com	&	43	&	vinmec.com	&	77	&	revolutionehr.com		\\
10	&	nhs.uk	&	44	&	goodrx.com	&	78	&	conobie.jp		\\
11	&	aarp.org	&	45	&	altibbi.com	&	79	&	verywellmind.com		\\
12	&	activebeat.com	&	46	&	popmama.com	&	80	&	familyandpets.com		\\
13	&	clevelandclinic.org	&	47	&	questdiagnostics.com	&	81	&	doctoralia.com.mx		\\
14	&	athenahealth.com	&	48	&	webteb.com	&	82	&	drogasil.com.br		\\
15	&	medlineplus.gov	&	49	&	uptodate.com	&	83	&	medicinenet.com		\\
16	&	1mg.com	&	50	&	hellosehat.com	&	84	&	myupchar.com		\\
17	&	menshealth.com	&	51	&	janeapp.com	&	85	&	medicare.gov		\\
18	&	msdmanuals.com	&	52	&	klikdokter.com	&	86	&	superdrug.com		\\
19	&	apteka.ru	&	53	&	practicefusion.com	&	87	&	consultaremedios.com.br		\\
20	&	doctoralia.com.br	&	54	&	phreesia.com	&	88	&	edh.tw		\\
21	&	myfitnesspal.com	&	55	&	eatthis.com	&	89	&	sehatq.com		\\
22	&	facty.com	&	56	&	simplepractice.com	&	90	&	myprotein.com		\\
23	&	who.int	&	57	&	healthygem.com	&	91	&	jtc.doctorqube.com		\\
24	&	alodokter.com	&	58	&	medscape.com	&	92	&	fda.gov		\\
25	&	drugs.com	&	59	&	practo.com	&	93	&	eclinicalworks.com		\\
26	&	halodoc.com	&	60	&	fahorro.com	&	94	&	doctissimo.fr		\\
27	&	babycenter.com	&	61	&	healthgrades.com	&	95	&	rlsnet.ru		\\
28	&	uworld.com	&	62	&	abczdrowie.pl	&	96	&	health.gov.au		\\
29	&	fitbit.com	&	63	&	prodoctorov.ru	&	97	&	bupa.com.au		\\
30	&	womenshealthmag.com	&	64	&	medonet.pl	&	98	&	hotdoc.com.au		\\
31	&	drogaraia.com.br	&	65	&	chemistwarehouse.com.au	&	99	&	priceline.com.au		\\
32	&	my-personaltrainer.it	&	66	&	leafly.com	&	100	&	ama.com.au		\\
33	&	login.nhs.uk	&	67	&	ecwcloud.com	&		&			\\
34	&	vidal.ru	&	68	&	health.clevelandclinic.org	&		&			\\
\bottomrule
\end{tabular}
\end{table}

\begin{longtable}{l|l}
\caption{The Survey Template}
\label{tab:template}
% \small
%  \hline\noalign{\smallskip}
%   Inlier& AUROC \uparrow&FPR at 95\% TPR \downarrow&Detection \,Error \downarrow&AUPR-In \uparrow&AUPR-Out \uparrow\\ 
% %  \midrule
%  \noalign{\smallskip}\cline{2-6}\noalign{\smallskip}
%  Classes&\multicolumn{5}{c}{GPND/CRAAE} \\ 
\hline
\textbf{Steps}& \textbf{Action}\\
\hline
1& Visit the homepage of the website.\\
\hline
& Please enter the domain of the website to google search engine.\\
\hline
&Note if there are privacy nudges on the homepage of this website.\\
\hline
1.1& Did you see privacy nudges?\\
\hline
&If Yes for 1.1, then answer following questions for step 1.1.\\
\hline
1.1.1& Where on a window screen these nudges are displayed? \\
1.1.2& What types of triggers are available? \\
1.1.3& What types of privacy nudges they are pushing?\\ 
1.1.4& What types of privacy actions  they are asking for?\\
1.1.5& Whether  there are detailed explanations of the meanings and results for those action options ? \\
\hline
&Note if there are privacy notices on the homepage of this website.\\
\hline
1.2& Did you see  privacy notices? \\
\hline
&If Yes for 1.3, then answer following questions for step 1.2.\\
\hline
1.2.1& Where on a window screen these notices are displayed? \\
1.2.2& What types of triggers are available? \\
1.2.3& What types of privacy information they are noticing? \\
\hline
&Note if there are privacy policy related button on the homepage of this website.\\
\hline
1.3& Whether there is privacy policy button on the website before log in? \\
\hline
&If Yes to 1.3, then answer following questions for step 1.3.\\
\hline
1.3.1& Where on a window screen the privacy policy button is displayed?\\
1.3.2& How many clicks are needed to access the privacy policy?\\
1.3.3& Is the privacy policy available in various languages?\\ 
1.3.4 &Whether the privacy policy contains contents to guide reading? \\
1.3.5& Whether the privacy policy contains  privacy setting options? \\
1.3.6& Whether the privacy policy contains privacy setting links?\\ 
1.3.7& Whether the privacy policy contains clear privacy setting guidance? \\
1.3.8& Which regulations this privacy policy follows?\\
1.3.9 & Which country this website belongs to (check the contact address of this website)? \\
\hline

&Note if there are privacy setting button on the website before log in.\\
\hline
1.4 &Whether there is privacy setting button on the website before log in? \\
\hline
&If Yes to 1.4, then answer following questions for step 1.4\\
1.4.1 &Where on a window screen the privacy setting button is displayed? \\
1.4.2& How many clicks are needed to access the privacy setting options?\\
1.4.3 &Is the privacy setting available in various languages? \\
1.4.4& Which aspects of privacy settings are covered? \\
\hline
\hline
2.& Create a user account for the website using an alias and email address provisioned for this analysis.\\
\hline
&Is there an option on the website to create a user account?\\
\hline
& If Yes for 2, then create a user account\\
\hline
2.1 &Did you see privacy nudges?\\
\hline
&If Yes for 2.1, then answer following questions for step 2.1.\\
\hline
2.1.1& Where on a window screen these nudges are displayed?\\
2.1.2& What types of triggers are available?\\
2.1.3& What types of privacy nudges they are pushing?\\
2.1.4& What types of privacy actions  they are asking for?\\
2.1.5& Whether  there are detailed explanations of the meanings and results for those action options ? \\
\hline
2.2& Did you see  privacy notices?\\
\hline
&If Yes for 2.2, then answer following questions for step 2.2.\\
\hline
2.2.1& Where on a window screen these notices are displayed?\\
2.2.2 &What types of triggers are available? \\
2.2.3 &What types of privacy information they are noticing?\\
\hline
2.3& Did you see privacy policy during creating an user account?\\
&If Yes to 2.3, then answer following questions for step 2.3.\\
\hline
2.3.1& Where on a window screen the privacy policy  is displayed?\\
\hline
2.4& Whether we can do privacy setting during creating an user account? \\
\hline
&If Yes to 2.4, then answer following questions for step 2.4.\\
\hline
2.4.1& Where on a window screen the privacy setting is displayed?\\ 
2.4.2& What types of triggers are available? \\
2.4.3 &Is the privacy setting available in various languages?\\
2.4.4& Which aspects of privacy settings are covered? \\
\hline
\hline
3 & Visit the website with log-in status.\\
% \hline
% 3.1 &Did you see privacy nudges? \\
% \hline
% &If Yes for 3.1, then answer following questions for step 3.1.\\
% \hline
% 3.1.1 &Where on a window screen these nudges are displayed? \\
% 3.1.2 &What types of triggers are available?\\
% 3.1.3& What types of privacy actions  they are asking for?\\
% 3.1.4& What types of privacy nudges they are pushing?\\
% 3.1.5& Whether  there are detailed explanations of the meanings and results for those action options ? \\
% \hline
% 3.2& Did you see  privacy notices? \\
% \hline
% &If Yes for 3.2, then answer following questions for step 3.2.\\
% \hline
% 3.2.1& Where on a window screen these notices are displayed?\\
% 3.2.2 &What types of triggers are available? \\
% 3.2.3 &What types of privacy information they are noticing?\\
\hline
3.1 &Whether there is privacy setting in the account setting after log in? \\
\hline
&If Yes to3.1, then answer following questions for step 3.1.\\
\hline
3.1.1& Where on a window screen the privacy setting button is displayed? \\
3.1.2& How many clicks are needed to access the privacy settings?\\
3.1.3& Is the privacy setting available in various languages?\\
3.1.4& Which aspects of privacy settings are covered? \\

\noalign{\smallskip}\hline\
%  \bottomrule

\end{longtable}
%\end{center}
% \end{table}
